# Supplementary material for: Dynamic stall of a hydrofoil with tubercles in surface gravity waves
Source: arXiv:2508.13329 source file (2025-08-18)
Supplement: Supplementary file 1 [file SuppMat_Foil_wave_R0.pdf]

# Supplemental Materials of
# "Dynamic stall of a hydrofoil with tubercles in surface gravity waves"

Guillaume Ricard[1,2], Gunnar Jacobi[1], Daniele Fiscaletti[1], Abel-John Buchner[2]
[1] *Department of Maritime & Transport Technology, Faculty of Mechanical Engineering, Delft University of Technology, Delft, The Netherlands*
[2] *Department of Process & Energy, Faculty of Mechanical Engineering, Delft University of Technology, Delft, The Netherlands*

In this Supplemental Material, we present additional results regarding force measurements for the straight-leading-edge hydrofoil with different wave lengths (Sect.S1), their corresponding probability density function (sect.S2) and the different component of the steady-state model (Sect.S3). We also show the effects of different wave amplitudes on the tubercled hydrofoil (Sect.S4) as well as the corresponding probability density functions (Sect.S5). Finally, the tangential velocity is discussed for other wave forcing (Sect.S6).

## S1. OTHER WAVELENGTHS FOR THE STRAIGHT LEADING-EDGE HYDROFOIL

In this section, the variation of $\eta(t)$, $F_x(t)$ and $F_z(t)$ for $\lambda = 2$ m (Fig.S1) and $\lambda = 6$ m (Fig.S2) for different wave amplitudes are plotted. Similar results to those discussed in the main paper for $\lambda = 4$ m are observed.

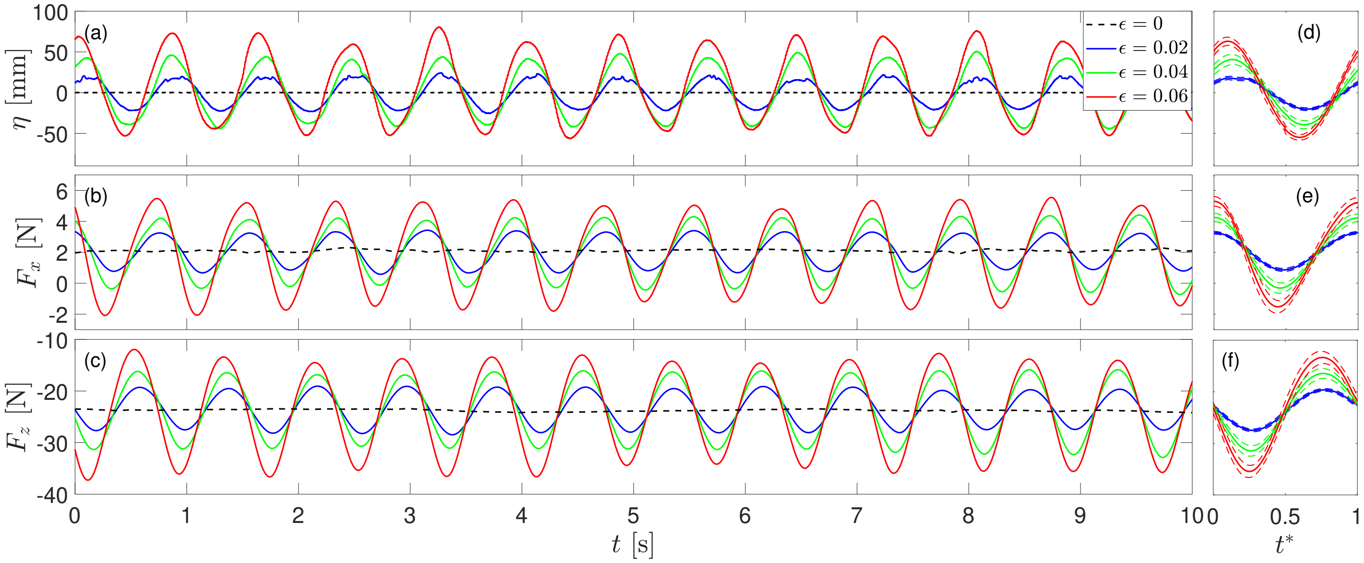


Figure S1. Time history of the surface elevation $\eta(t)$ (a), the horizontal force component $F_x(t)$ (b), and the vertical force component $F_z(t)$ (c), $\lambda = 2$ m and different waves amplitude $\epsilon = 0$ (black dashed lines), 0.02 (blue solid lines), 0.04 (green solid lines) and 0.06 (red solid lines). (d,e,f) Same but with phase averaged data over 40 wave periods, dashed lines correspond to the standard deviation of the average.

## S2. PROBABILITY DENSITY FUNCTIONS FOR THE STRAIGHT-LEADING-EDGE HYDROFOIL

The signals observed previously can be analysed using their normalised probability density function (PDF), see Fig.S3, defined with $\langle X \rangle$ the time average and $\sigma_X$ the standard deviation of a variable $X$. For the waves with weak intensity (small wave length $\lambda = 2$ m or small steepness $\epsilon = 0.02$), two distinct peaks characteristic of linear sinusoidal variations emerge for $\eta$, $F_x$ and $F_z$. For the waves with strong intensity, typically $\lambda = 4$ m and $\epsilon = 0.06$, the nonlinearity of the wave appears as they tend to go up more than they go down (dissymmetry of $PDF(\eta)$). A third peak appears on the $PDF(F_x)$ corresponding to the nonlinear fluctuation observed on $F_x(t)$ and the positive peak of $PDF(F_z)$ is much larger as $F_z(t)$ remains elevated (i.e., at its minimal lift) for a longer fraction of the wave period.

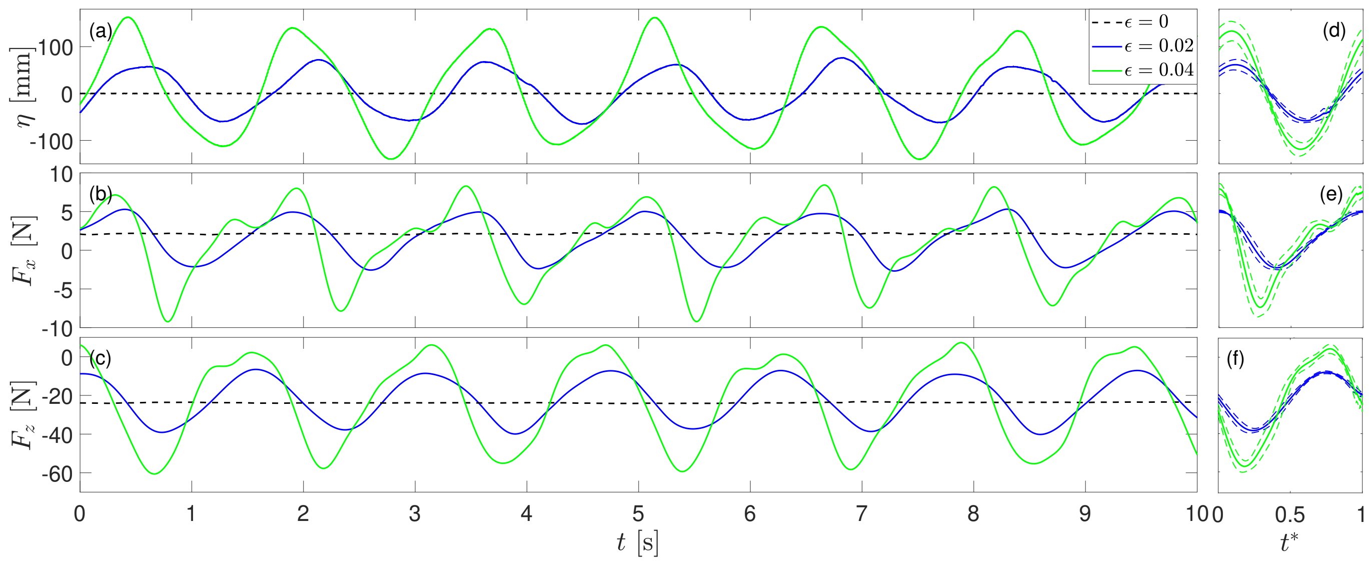


Figure S2. Time history of the surface elevation $\eta(t)$ (a), the horizontal force component $F_x(t)$ (b), and the vertical force component $F_z(t)$ (c), $\lambda = 6$ m and different waves amplitude $\epsilon = 0$ (black dashed lines), 0.02 (blue solid lines) and 0.04 (green solid lines). (d,e,f) Same but with phase averaged data over 40 wave periods, dashed lines correspond to the standard deviation of the average.

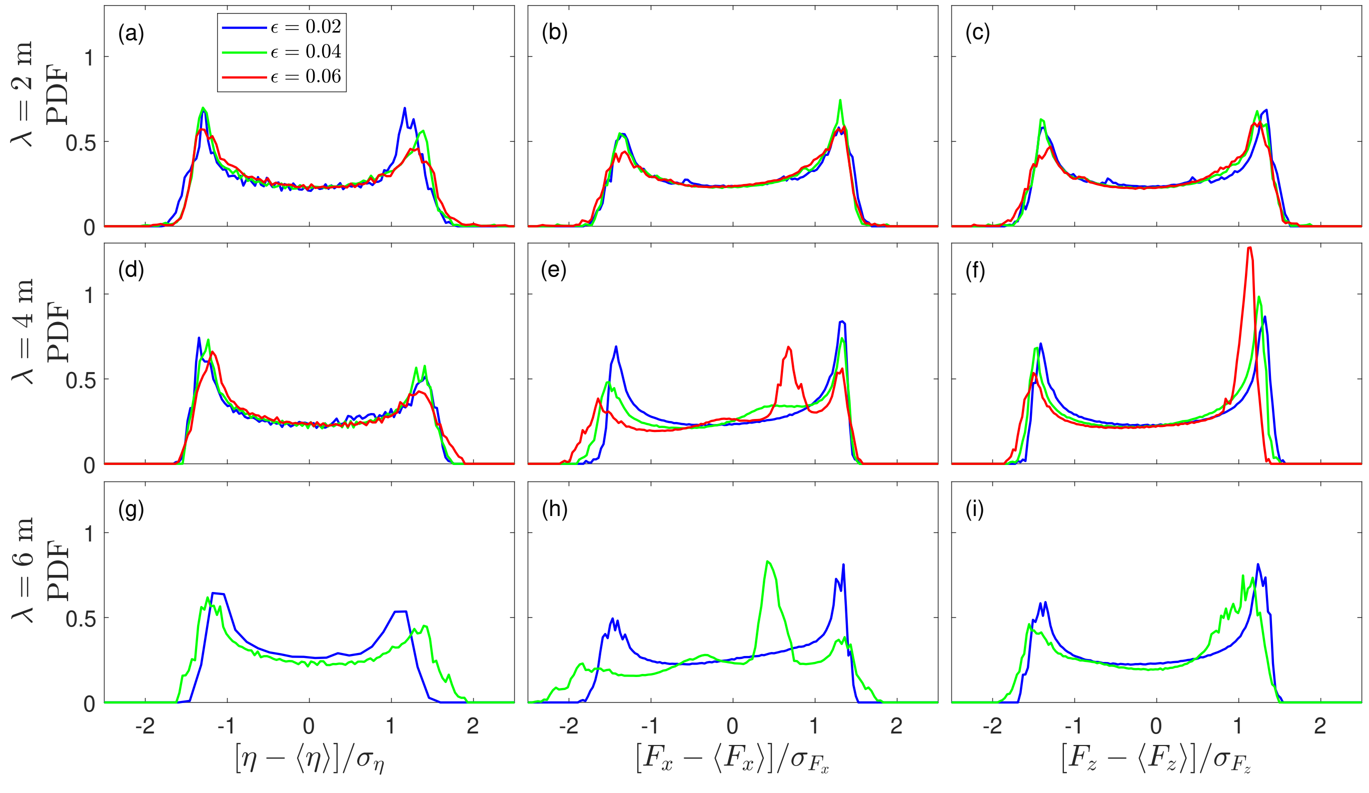


Figure S3. Normalised probability density functions of the surface elevation $\eta(t)$ (a,d,g), the horizontal forces $F_x$ (b,e,h) and the vertical forces $F_z$ (c,f,i), for $\lambda = 2$ m (a-c), $\lambda = 4$ m (d-f) and $\lambda = 6$ m (g-i), and for different waves amplitudes $\epsilon = 0.02$ (blue), 0.04 (green) and 0.06 (red).

## S3. STEADY-STATE MODEL

In Fig.S4, we plot the decomposition of the theoretical model of Eq.2.3 in the main text for $\lambda = 4$ m and (a,b) $\epsilon = 0.02$ and (c,d) $\epsilon = 0.06$. The minimal values of $F_x$ that emerge at large angle of attack are clearly dominated by inertia effects, whereas $F_z$ is mostly dominated by lift (and a small component of drag).

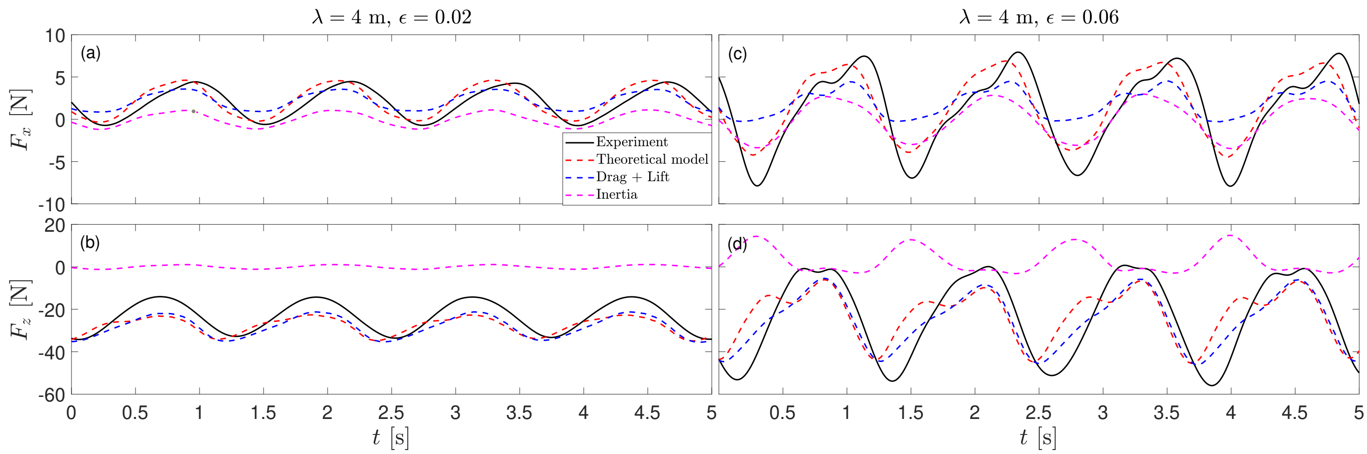


Figure S4. Decomposition of the theoretical model of the force variations (a,c) $F_x(t)$ and (b,d) $F_z(t)$, for $\lambda = 4$ m and (a,b) $\epsilon = 0.02$ and (c,d) $\epsilon = 0.06$. Experimentally measured values are plotted as solid black lines and the theoretical prediction as dashed lines: drag + lift component (blue), inertia (magenta) and the total model (red).

## S4. OTHER WAVE AMPLITUDE FOR THE TUBERCLES AND STRAIGHT LEADING-EDGE HYDROFOILS

In this section, the variation of $\eta(t)$, $F_x(t)$ and $F_z(t)$ for $\lambda = 4$ m and $\epsilon = 0.02$ (Fig.S5) and $\epsilon = 0.04$ (Fig.S5) is shown. Similar results to those discussed in the main paper for $\epsilon = 0.06$ m are observed, but with lower intensity.

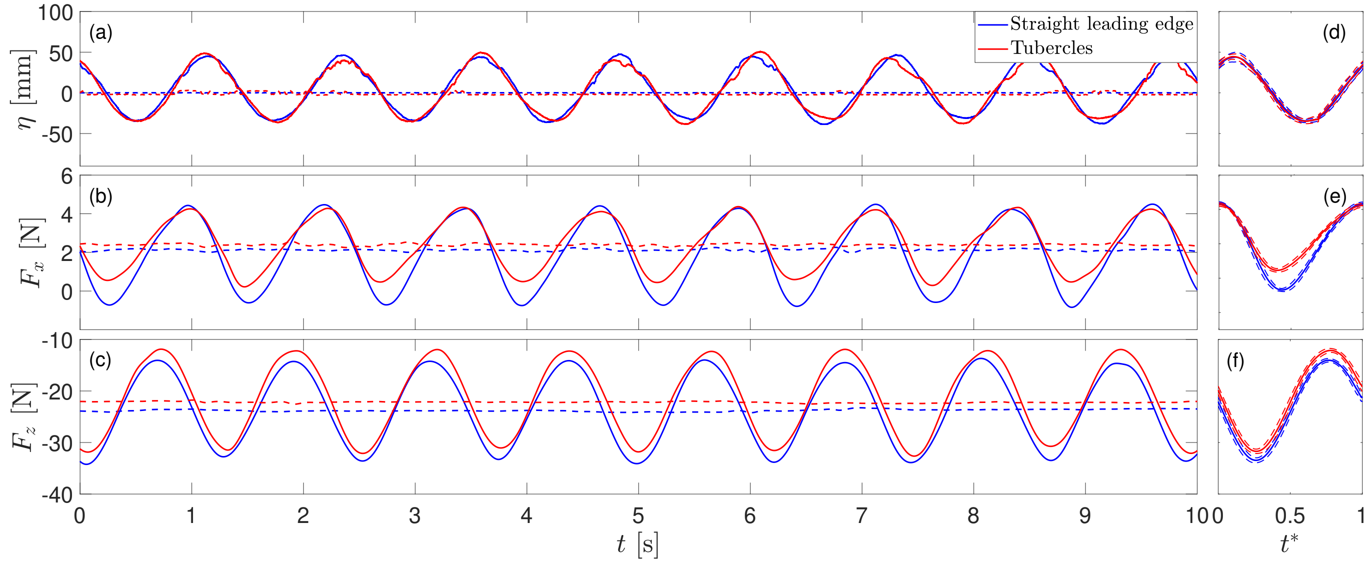


Figure S5. Time history of the surface elevation $\eta(t)$ (a), of the horizontal forces $F_x(t)$ (b) and of the vertical forces $F_z(t)$ (c), for $\lambda = 4$ m and $\epsilon = 0.02$ for the regular hydrofoil with straight leading edge (blue solid lines) and the one with tubercles (red solid lines). (d,e,f) Same but with phase averaged over 40 wave periods, dashed lines correspond to the standard deviation of the average.

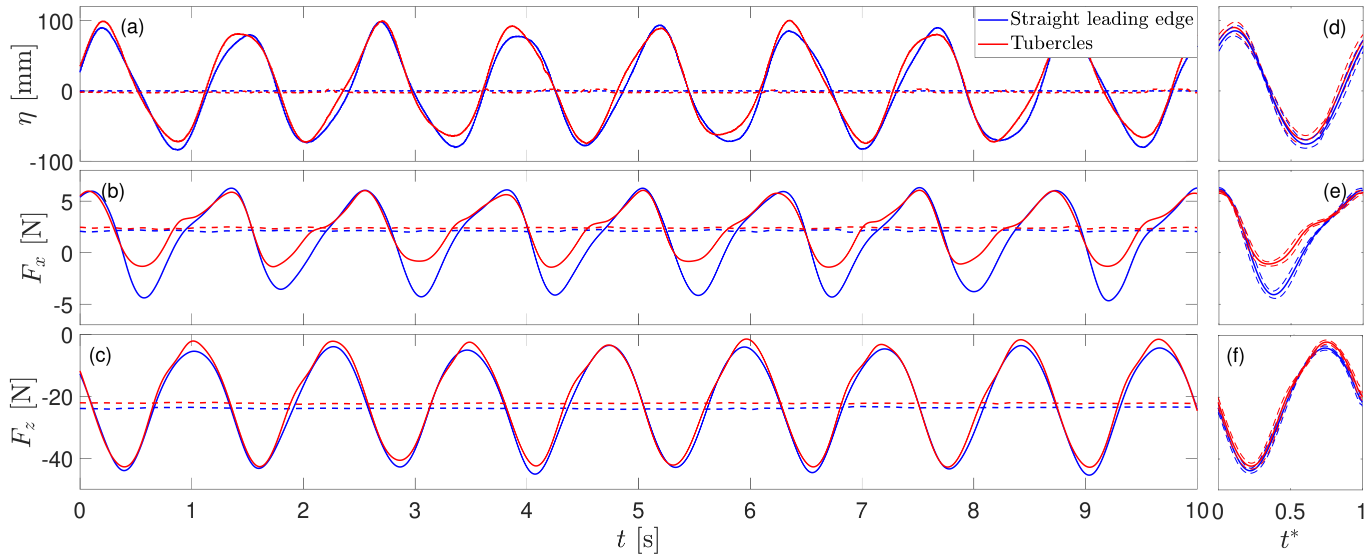


Figure S6. Time history (a) of the surface elevation $\eta(t)$, (b) of the horizontal forces $F_x(t)$ and (c) of the vertical forces $F_z(t)$, for $\lambda = 4$ m and $\epsilon = 0.04$ for the regular hydrofoil with straight leading edge (blue solid lines) and the one with tubercles (red solid lines). Same, but (d,e,f) with phase averaged over 40 wave periods, dashed lines correspond to the standard deviation of the average.

## S5. PROBABILITY DENSITY FUNCTION FOR THE TUBERCLED AND STRAIGHT-LEADING-EDGE HYDROFOILS

The probability density functions of the previous signals are then computed for $\lambda = 4$ m for different wave amplitudes and for the two hydrofoils in Fig.S7. The effect of tubercles is only observable when $\epsilon \geq 0.04$. For $F_x$ the negative peak is brought closer to 0 as drag is increased by the presence of an attached vortex (see main paper) and a third peak tends to be closer to 0 as the temporal variations of $F_x$ are modified. For $F_z$, tubercles decrease the time spent at its maximal value, resulting in a significant decrease of the positive peaks on $PDF(F_z)$.

## S6. OTHER WAVE AMPLITUDE FOR TANGENTIAL VELOCITY

The tangential velocity of the flow along the suction surface of each hydrofoil function of space and time is plotted in Fig.S8 for $\lambda = 4$ m, $\epsilon = 0.04$ and in Fig.S9 for $\lambda = 6$ m and $\epsilon = 0.04$. Similar dynamics to the one described in the main paper for $\lambda = 4$ m and $\epsilon = 0.06$ are here evidenced. However, the phenomena are observed with less intensity for $\lambda = 4$ m, $\epsilon = 0.04$ in Fig.S8. No leading-edge separation is observed for the straight-leading-edge case [Fig.S8 (a)] and the zones of flow separation are smaller for the tubercled hydrofoil [Fig.S8 (b-d)]. On the other hand, more intensity in the stall process emerges in Fig.S9 for $\lambda = 6$ m and $\epsilon = 0.04$. An actual reverse flow appears along the straight-leading-edge hydrofoil [zone B, Fig.S9 (a)]. For the tubercled hydrofoil, the areas of accumulation of vorticity [zone C, Fig.S9 (c,d)] and of stall [zone D, Fig.S9 (b-d)] are much larger compared to the case with $\lambda = 4$ m and $\epsilon = 0.06$ presented in the main paper.

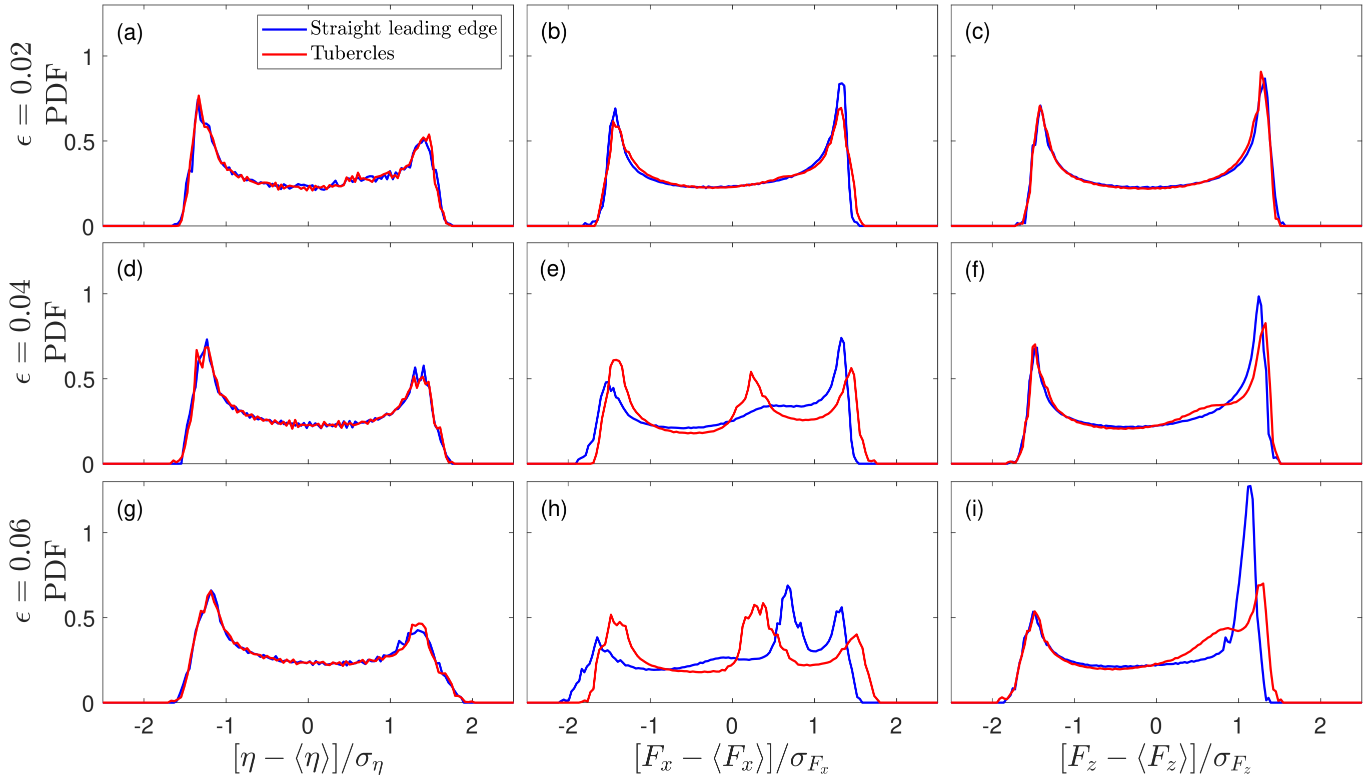


Figure S7. Normalised probability density functions of (a,d,g) the surface elevation $\eta(t)$, (b,e,h) the horizontal forces $F_x$, and (c,f,i) the vertical forces $F_z$, for (a,c) $\lambda = 4$ m and $\epsilon = 0.02$, (d-f) $\epsilon = 0.04$ and (g-i) $\epsilon = 0.06$, for the regular hydrofoil with straight leading edge (blue solid lines) and the one with tubercles (red solid lines).

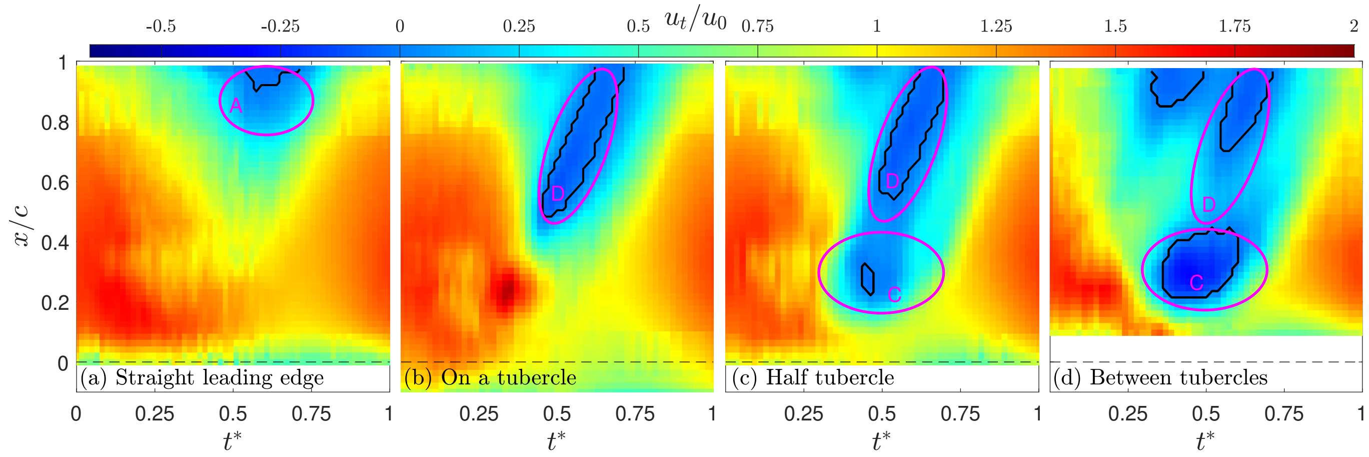


Figure S8. Spatio-temporal variations of the non-dimensional phase-averaged velocity, $u_t/u_0$, tangent to the hydrofoil suction surface at non-dimensional times $t^* \in [0, 1]$ for $\lambda = 4$ m and $\epsilon = 0.04$. The two cases (a) straight leading edge and (b-d) with tubercles are shown. Shows the measurement plane (b) on a tubercle peak, (c) halfway between tubercle peak and trough, and (d) at the trough between tubercles. Black solid curves delimit spatio-temporal regions in which $u_t < 0$. Alphabetically-labelled magenta ellipses indicate zones of interest to ease description.

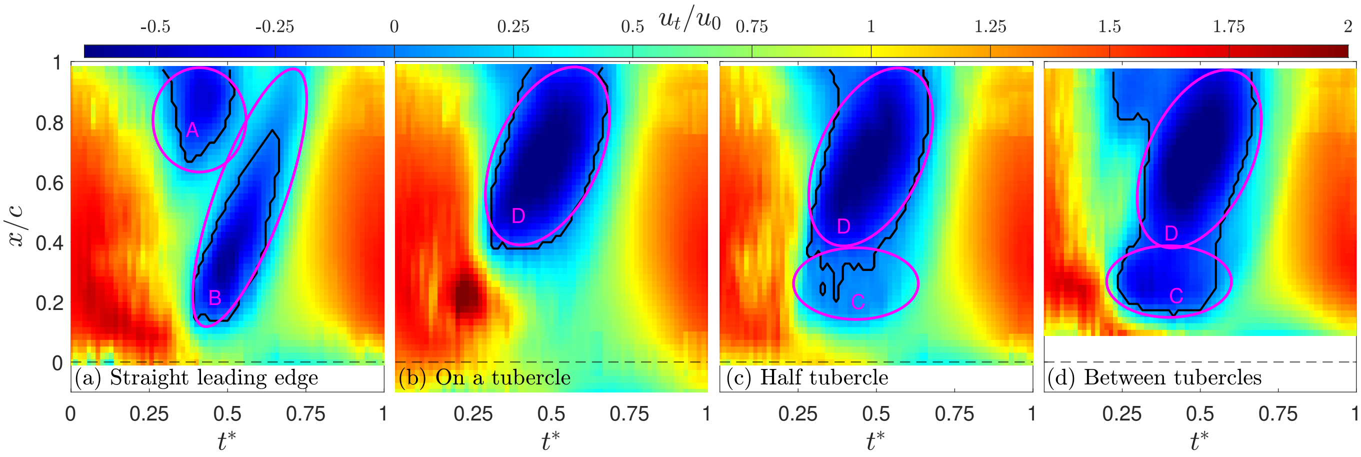


Figure S9. Spatio-temporal variations of the non-dimensional phase-averaged velocity, $u_t/u_0$, tangent to the hydrofoil suction surface at non-dimensional times $t^* \in [0, 1]$ for $\lambda = 6$ m and $\epsilon = 0.04$. The two cases (a) straight leading edge and (b-d) with tubercles are shown. Shows the measurement plane (b) on a tubercle peak, (c) halfway between tubercle peak and trough, and (d) at the trough between tubercles. Black solid curves delimit spatio-temporal regions in which $u_t < 0$. Alphabetically-labelled magenta ellipses indicate zones of interest to ease description.
